# Supplementary material for: A robust parallel algorithm for combinatorial compressed sensing
Source: arXiv:1704.09012 source file (2017-04-28)
Supplement: Supplementary file 1 [file appendix.tex]

\appendix
\section{Appendix}

% Randomised-Robust-l0
\begin{small}
	\begin{algorithm}
   \KwData{$A \in \expander$; $y \in \R^m$; $\alpha \in (1, d]$; $\sigma_s, \sigma_n \in (0,\infty)$}
   \KwResult{ $\hat x \in \R^n$ $\st$ $ \hat x \approx x$ satisfies $y = A \hat x$}
    $\hat x \leftarrow 0$, $r \leftarrow y$\;
    Let $p_z(\cdot)$, $p_e(\cdot)$ be defined according to \eqref{eqn:bayesian_pz} and \eqref{eqn:bayesian_pe}.
    $\hat x \gets 0$\;
    $\hat r \gets r$\;
		\While{not converged}{
		  \For{$j \in [n]$}{
        %$v \leftarrow r_{\Nc(j)}$\;
		    \For{$i \in [d]$}{
          \If{$B_{p_z(r_{\Nc(i)})}$}{
            \If{$\sum_{i=1}^d B_{p_e(r_{\Nc(i)} - r_{\Nc(j)})} - B_{p_z(r_{\Nc(i)})} \ge \alpha $ and $\norm{r_{\Nc(j)}-u}_1 \le \norm{r_{\Nc(j)}}_1$}{
              $\hat x_j \leftarrow \hat x_j + u$\;
              $r_{\Nc(j)} \leftarrow r_{\Nc(j)} - u$\;
            }
          }
        }
		    $\hat x \gets \Hc_k(\hat x)$\;
		    $r \gets y- A\hat x$\;
      }
    }
  \caption{Randomised Robust-$\ell_0$}
  \label{alg:rand-robust-l0}
	\end{algorithm}
\end{small}

\subsection{Parameter Estimation}
While most CS algorithms need to know the sparsity $k$ of $x$ in advance, our algorithm also needs to know the magnitude of the noise compared to the signal. 
It is thus necessary to find a method that can estimate those parameters from a vector $y$.
We propose two methods that can be used to estimate the parameters.
\paragraph{Quantile-based method to estimate noise levels}
This simple but fast method assumes that we know the sparsity and the signal strength (assume again $\sigma_s=1$ for simplicity).
Begin by sorting $\abs{\hat y_i}$ (increasing) and call the sorted vector $\bar y$. 
From the zero-probability calculations above, we know that there will be approximately $L = m\exp(-\tau)$ zero entries in $y$. 
Assuming very small noise, it is reasonable to assume that the first $L$ values in $\bar y$ are just from $\eta$,
hence a first idea is to just take the empirical standard deviation of these first $L$ values. 
However, if only a few of the values are not just from $\eta$ but also correspond to non-zeros in $y$, then this estimate will be much too big.
Hence we propose to instead take the $l_0=\lceil L/2\rceil$ smallest values in $\bar y$ and dividing it by $0.675$, i.e.
\begin{equation}
	\hat \sigma_{n,(0)} = \frac{\bar y_{l_0}}{0.675}.
\end{equation}
This is based on the fact that for a Gaussian random variable the 50\% quantile of its absolute values is approximately $0.675$ standard deviations from the mean.
However, when the noise is similar to the signal strength, then a significant number of signal values will be smaller than $\bar y_{l_0}$, and thus skewing the estimate and making it too small.
A correction is given by 
\begin{equation}
	\hat \sigma_{n,(1)} = \frac{\bar y_{l_1}}{0.675},
\end{equation}
where
\begin{equation}
	l_1 = \left\lceil (m-L) 2\left(\Phi(l_0,0,\sqrt{2\hat \sigma^2_{n,(0)} + \frac{\tau}{1-\exp(-\tau)}})-0.5\right) \right\rceil.
\end{equation}
This idea can be iterated, giving more and more accurate estimates for $\sigma_n$.
\begin{figure}%[H]
	\centering
	\includegraphics[width=0.49\linewidth]{figures/noise_estimate_delta=0_5_rho=0_1.eps}
	\includegraphics[width=0.49\linewidth]{figures/noise_estimate_delta=0_5_rho=0_3.eps}
	\caption{Estimates for $\sigma_n$ using the quantile based approach. Left: $\rho=0.1$, right: $\rho=0.3$.}
	\label{fig:noise-estimate-quantile-based}
\end{figure}
In Figure~\ref{fig:noise-estimate-quantile-based} we can see that the estimate works extremely well for smaller $\rho$ and is decent for larger $\rho$ up to noise levels of about $\sigma_n=10^{-1}$. 
This is satisfying as we can not really expect good recovery for noise larger than this anyway.
\paragraph{Using the EM-Algorithm to Estimate Noise Level, Signal Level and Sparsity}
In the derivation for the zero- and equal-probabilities we have approximated $y$ with a Gaussian Mixture Model (GMM), containing some entries that are only noise, and some entries that consist of signal and noise.
Hence if we are able to fit a GMM to $y$ we immediately know the noise level and we can use our knowledge about the structure of $x$ and $A$ to derive $\sigma_s$ and the sparsity $k$.

Fixing the mean of the noise and the signal to zero, the EM-Algorithm outputs $\sigma_1$, $\sigma_2$ and a fraction $\gamma$ of values that belong to the normal distribution with standard deviation $\sigma_1$.
Assume without loss of generality that $\sigma_1\le \sigma_2$, than the relationship between $\gamma$ and $\tau$ introduced earlier is given by $\gamma=\exp(-\tau)$ and hence we can infer $\rho = -\log(\gamma)/d$.
Note that earlier (cf. \eqref{eqn:10301623}) we derived the standard deviation of those entries in $\hat y$ that correspond to a non-zero entry in $y$, and hence we can solve for $\sigma_s$, $\sigma_n$ and $\rho$ by solving
\begin{equation}
	\begin{aligned}
		\rho &= -\log(\gamma)/d\\
		\sigma_n & = \sigma_1\\
		\sigma_2 &= \sqrt{\sigma_n^2 + \sigma^2_s \tau/(1-\exp(-\tau))}.
	\end{aligned}
\end{equation}
\begin{remark}
	Note that the EM Algorithm will also output a likelihood for each entry in $\hat y$ whether it is just noise or from signal. 
	This likelihood can be used in the first iteration of the l0-decoding algorithm.
\end{remark}
In practice we do not simply use the entry in the residual as the update but the mean over all entries in the residual that have been classified as equal to that entry (up to noise).
This leads to errors in $x$ that are potentially smaller than the standard deviation of the noise.

\begin{figure}%[H]
	\centering
	\includegraphics[width=0.8\linewidth]{figures/runtime_over_n_delta=0_4_rho=0_1_sigma=1e-03-eps-converted-to.pdf}
	\caption{Run time of recovery algorithms as $n$ increases.}
	\label{fig:runtime-scaling}
\end{figure}

%%% rho vs noise

\begin{figure}%[H]
	\centering
	\includegraphics[width=0.8\linewidth]{figures/phase_transitions/rho_vs_noise_probs_robust-l0-adaptive-trans-crop.pdf}
	\includegraphics[width=0.8\linewidth]{figures/phase_transitions/rho_vs_noise_time_robust-l0-adaptive-trans-crop.pdf}
	\caption{Phase transition varying $\sigma$ for deterministic-robust-$\ell_0$}
	\label{fig:varying_sigma_det_rob_l0}
\end{figure}

\begin{figure}%[H]
	\centering
	\includegraphics[width=0.8\linewidth]{figures/gaga/rho_vs_noise_probs_robust-l0-crop.pdf}
	\includegraphics[width=0.8\linewidth]{figures/gaga/rho_vs_noise_time_robust-l0-crop.pdf}
	\caption{Phase transition varying $\sigma$ for robust-$\ell_0$}
	\label{fig:varying_sigma_rob_l0}
\end{figure}

\begin{figure}%[H]
	\centering
	\includegraphics[width=0.8\linewidth]{figures/gaga/rho_vs_noise_probs_robust-l0-trans-crop.pdf}
	\includegraphics[width=0.8\linewidth]{figures/gaga/rho_vs_noise_time_robust-l0-trans-crop.pdf}
	\caption{Phase transition varying $\sigma$ for robust-$\ell_0$}
	\label{fig:varying_sigma_rob_l0}
\end{figure}

\begin{figure}%[H]
	\centering
	\includegraphics[width=0.8\linewidth]{figures/gaga/rho_vs_noise_probs_ssmp-robust-crop.pdf}
	\includegraphics[width=0.8\linewidth]{figures/gaga/rho_vs_noise_time_ssmp-robust-crop.pdf}
	\caption{Phase transition varying $\sigma$ for SSMP-robust-$\ell_0$}
	\label{fig:varying_sigma_det_ssmp_robust}
\end{figure}
